# Supplementary material for: Statistical Analysis of the Role of Invariant Manifolds on Robust Trajectories
Source: arXiv:2409.19905 source file (2024-09-30)
Supplement: Supplementary file 1 [file appendix.tex]

\section*{Appendix}

\ifthenelse{\boolean{includefigures}}
{
    \begin{figure}[!htbp]
        \centering
        \begin{tikzonimage}[width=0.6\linewidth, keepaspectratio=True]{"rob_vs_nonrob_closest_manifold_start.png"}%[tsx/show help lines]
        \Large
        \node[fill=white, opacity=0.0, text opacity=1, anchor=south, rotate=90] at (-0.025,0.815) {\textbf{Non-Robust}};
        \node[fill=white, opacity=0.0, text opacity=1, anchor=south, rotate=90] at (-0.025,0.36) {\textbf{Robust}};
        \end{tikzonimage}
        \caption{$\hat{d}_T$ at various energy levels sorted by $\mathcal{P}(x)$ and $\mathcal{P}^{-1}(x)$ for the non-robust and the robust solutions (sorted by $\tau$).}
        \label{fig: closest_manifold_start}
    \end{figure}
}
{
    % Do nothing
}

\ifthenelse{\boolean{includefigures}}
{
    \begin{figure}[!htbp]
        \centering
        \begin{tikzonimage}[width=0.95\linewidth, keepaspectratio=True]{"rob_vs_nonrob_closest_manifold_duration.png"}%[tsx/show help lines]
        \Large
        \node[fill=white, opacity=0.0, text opacity=1, anchor=south, rotate=90] at (0.25,0.87) {\textbf{Non-Robust}};
        \node[fill=white, opacity=0.0, text opacity=1, anchor=south, rotate=90] at (-0.01,0.39) {\textbf{Robust}};
        \end{tikzonimage}
        \caption{$\hat{d}_T$ at various energy levels sorted by $\mathcal{P}(x)$ and $\mathcal{P}^{-1}(x)$ for the non-robust and the robust solutions (sorted by $\Delta \tau$).}
        \label{fig: closest_manifold_duration}
    \end{figure}
}
{
    % Do nothing
}

% \ifthenelse{\boolean{includefigures}}
% {
%     \begin{figure}
%         \centering
%         \includegraphics[width=\linewidth, keepaspectratio=True]{rob_vs_nonrob_closest_manifold_duration.png}
%         \caption{$\hat{d}_T$ at various energy levels sorted by $\mathcal{P}(x)$ and $\mathcal{P}^{-1}(x)$ for the non-robust and the robust solutions (sorted by $\Delta \tau$).}
%         \label{fig: closest_manifold_duration}
%     \end{figure}
% }
% {
%     % Do nothing
% }
